# Supplementary material for: Bridging the Gap Between Ideal and Real-world Evaluation: Benchmarking AI-Generated Image Detection in Challenging Scenarios
Source: arXiv:2509.09172 source file (2025-09-11)
Supplement: Supplementary file 1 [file 7_appendix.tex]

\clearpage
\setcounter{page}{1}
\maketitlesupplementary

\setcounter{section}{0}

\section*{Supplementary Overview}
\addcontentsline{toc}{section}{Supplementary Overview}
\textbf{Dataset:}  \url{https://zenodo.org/records/14963880}.

\noindent \textbf{Code:} \url{https://github.com/ChunXiaostudy/RRDataset}.

\noindent \textbf{Weights:} \url{https://zenodo.org/records/14991882}.

\noindent The following provides an overview of the content in each Appendix section:
\begin{itemize}
    \item \textbf{Section A}: Comprehensive Introduction of AI-Generated Image Detectors.
    \item \textbf{Section B}: Real-World Applications of Transmission and Re-digitization.
    \item \textbf{Section C}: Training Details.
    \item \textbf{Section D}: Additional Results for RRBench.
    \item \textbf{Section E}: Comparison of Human Attention Regions.
    \item \textbf{Section F}: Frequency Domain Analysis.
    \item \textbf{Section G}: Visualization of RRDataset.
    \item \textbf{Section H}: Further Discussion and Suggestion.
    \item \textbf{Section I}: Limitation of RRDataset and RRBench.

\end{itemize}

\section{Comprehensive Introduction of AI-Generated Image Detectors}
Based on the detection criteria, the methods for detecting AI-generated images can be broadly categorized into the following approaches: detection based on pixel-domain features, detection based on frequency-domain features, detection leveraging pre-trained model features, detection utilizing fused features, as well as rule-based detection methods.
Detection based on pixel-domain features of images identifies authentic or synthetic images through common patterns in pixel-level characteristics, which primarily encompasses approaches utilizing steganalysis features \cite{marra2018detection}, texture features \cite{Nataraj2019Detecting,goebel2020detection,qiao2023csc}, color features \cite{Chandrasegaran2022Discovering,uhlenbrock2024did}, local features \cite{chen2024single,karageorgiou2024any,cavia2024real}, reconstruction features \cite{he2021beyond,zhang2023diffusion,wang2023dire,lim2024distildire,luo2024lare,ricker2024aeroblade,ma2024exposing,chu2025fire,cazenavette2024fakeinversion,chen2024drct}, internal correlation features \cite{zhong2024patchcraft,tan2024rethinking,Chen2024IPD} and physical features \cite{Sarkar2024Shadows}. Besides, Tan et al. \cite{Tan2023Learning} first proposed a gradient-based detection method (LGrad) that employs gradient maps derived from pretrained CNN models. This method trains a binary classifier on gradient map datasets to distinguish AI-generated images from authentic ones. By eliminating the influence of image semantics on the detector, this approach effectively mitigates the model's dependency on training data. However, due to its reliance on specific pretrained architectures, LGrad demonstrates limited generalizability when applied to images generated by non-CNN-based models.

Detection based on frequency domain characteristics of images primarily identifies artificial patterns by analyzing common characteristics exhibited in the frequency domain of generated images. This approach typically converts images into spectrum maps for subsequent analysis through detection networks. Representative methods include: Discrete Fourier Transform (DFT)-based detection \cite{zhang2019detecting,durall2020watch,Dzanic2020Fourier, jeong2022bihpf, li2024masksim}, Discrete Cosine Transform (DCT)-based detection \cite{frank2020Leveraging,bonettini2021use,pontorno2024exploitation}, and Fast Fourier Transform (FFT)-based detection \cite{Jeong2022FingerprintNet}.
Detection based on pre-trained model features leverages large-scale models to accomplish detection tasks. Several research efforts directly utilize the powerful feature extraction capabilities of pre-trained models for detection \cite{Ojha2023Towards,cozzolino2024raising, gaintseva2024improving, yang2024text}. Notably, Ojha et al. \cite{Ojha2023Towards} employ the pre-trained CLIP model to extract image features for detector training, enabling the learning of more balanced decision boundaries and thereby enhancing the detector's generalization across different generative models. Koutlis and Papadopoulos \cite{koutlis2024leveraging} propose RINE, which extracts intermediate image representations from the CLIP image encoder, maps them into a learnable forgery-aware vector space, and incorporates a trainable module to predict the importance of each encoder layer. Other approaches focus on fine-tuning vision-language models \cite{wu2023generalizable, chang2023antifakeprompt, xu2024famsec,liu2024mixture,khan2024clipping,keita2024harnessing,keita2025bi,tan2024c2p} or large language models \cite{fan2024fake} for detection tasks. Among these, C2P-CLIP \cite{tan2024c2p} introduces class-agnostic prompts to reinforce the conceptual distinction between real and generated images through contrastive learning, while implementing CLIP fine-tuning via Low-Rank Adaptation (LoRA) \cite{hu2022lora} to develop a universal detector for generated images.
Detection methods based on fused features can be further categorized by modality quantity into single-modality fused feature detection methods and multi-modality fused feature detection methods. Single-modality fused feature detection methods refer to approaches that solely integrate different features within images, including pixel-domain feature fusion \cite{Ju2022Fusing, Ju2024GLFF,Xi2023AI,leporoni2024guided,raza2024mmganguard,baraldi2024contrasting}, frequency-domain feature fusion \cite{ liu2022Detecting,tan2024data}, hybrid pixel-frequency domain feature fusion \cite{liu2024forgeryaware,lanzino2024faster,meng2024artifact, wissmann2024whodunit}, and the integration of spatial features with semantic features in images \cite{yan2024sanity}. Multi-modality fused feature detection methods involve the fusion of features from diverse modalities such as images and texts \cite{sha2023defake,lin2024robust,yu2024semgir}. Notably, Sha et al. \cite{sha2023defake} focused on detecting text-to-image model generated content, revealing that generated images closer proximity to their prompt texts compared to real images. Leveraging this observation, they proposed DEFAKE, which concatenates CLIP-extracted textual and visual features to construct discriminative features for detection.
Rule-based detection methods typically leverage the differences in sensitivity between two categories of images to the same operations as the detection criterion. These approaches generally require no training process, and since the detection procedure does not rely on classifiers, the results tend to be unbiased \cite{ricker2024aeroblade,sha2024zerofake,choi2024hfi, tsai2024understanding}. 
In a distinct approach, Ricker et al. \cite{ricker2024aeroblade} proposed Aeroblade, which utilizes the reconstruction error of autoencoders combined with the Learned Perceptual Image Patch Similarity (LPIPS) metric to detect generated images.

In summary, regarding generative image detection, most studies employ model-based supervised learning, some utilize semi-supervised \cite{Jeon2020TGD} or unsupervised paradigms \cite{qiao2023csc}, few use instance-based approach to perform detection. The features such as noise patterns in the pixel domain and frequency domain, texture, color information, and mapping geometry have turned into detection cues. Some studies aim to enhance the generalization of detection methods when faced with different generative models. Besides, robustness against common image processing also becomes an aspect of evaluating detection methods.

\section{Real-World Applications of Transmission and Re-digitization}
AI-generated image detection fundamentally differs from traditional image classification tasks. A key distinction is that, for traditional classification tasks such as ImageNet1K, real-world applications typically involve photos captured directly by users or devices, such as autonomous vehicle cameras. However, with the rise of social media and other platforms, an image suspected to be AI-generated may have already undergone multiple rounds of transmission or even appeared in physical form.

In real-life scenarios, the images available for detection are often subjected to lossy internet transmission through social media platforms. Therefore, incorporating such transmitted images into the test set is crucial for a robust evaluation of detection algorithms.

Regarding re-digitization, we first present real-world applications of this process to explain why re-digitization is essential for AI-generated image detection. Re-digitization refers to the process of converting an existing digital image (e.g., stored in formats such as JPG or PNG) into a physical form (e.g., printing or displaying it on a screen) and then converting it back into a digital format through methods such as scanning or photography.

Re-digitization has numerous real-world applications, including the following:

\begin{itemize}
    \item Capturing photos of images displayed on devices, where exporting images is not permitted.
    \item Photographing screens to save images that are protected against direct downloads or screenshots in web pages or Apps.
    \item Scanning printed materials, such as newspapers or magazines, to create electronic versions of articles or images.
    \item Capturing projected content during presentations when direct access to slides is unavailable.
    \item Photographing artwork in museums or galleries where digital copies cannot be obtained, for documentation or personal use.
    \item Recording street art, graffiti, posters, or other outdoor artworks for preservation or documentation.
\end{itemize}
Therefore, detection algorithms must  adapt to diverse re-digitization processes, including scanned documents, photographed screens, or printed photographs. By incorporating these scenarios into benchmarks, we ensure that detection algorithms are practical and reliable across domains. Additionally, including re-digitized samples in benchmarks forces algorithms to learn more generalized features rather than relying solely on subtle artifacts in the original digital image. This enhances their performance in unknown environments and against emerging generative models.

\section{Training Details}
\noindent \textbf{Hardware and Environment:} 
All training and testing were conducted on a single NVIDIA RTX 4090 GPU using PyTorch 2.0.1.

\noindent \textbf{Training Details:} For all detectors, we adopted the training setup used in GenImage \cite{zhu2023genimage} and AIDE\cite{yan2024sanity}. Specifically, training was conducted on GenImageSD1.4, where a subset of SDv1-4 was used, consisting of 162,000 AI-generated images from SDv1-4 and 162,000 real images from ImageNet, with an additional 6,000 AI-generated and 6,000 real images reserved for validation.

For certain methods, such as CNNSpot \cite{wang2020cnn}, GramNet \cite{liu2020global}, DIRE \cite{wang2023dire} and DNF \cite{zhang2023diffusion}, only pretrained weights from the ProGAN dataset were available. Therefore, we replicated their respective training settings and data augmentation procedures to ensure thorough training. For methods already trained and validated on SDv1-4, we directly utilized their publicly released pretrained weights.

\noindent \textbf{Fine-Tuning Details} To provide a more comprehensive and realistic evaluation of each detector, we fine-tuned all 17 detection models using a subset of RRDataset-Original. Specifically, we selected 1,250 real images and 1,250 AI-generated images for training, with an additional 250 real and 250 AI-generated images for validation.

Fine-tuning was performed using a batch size of 64 for 5 epochs with the AdamW optimizer, starting with an initial learning rate of $5 \times 10^{-4}$. We employed a learning rate decay strategy and early stopping to optimize performance.

\noindent \textbf{VLM Prompt Selection:} To maximize the detection performance of VLMs, we manually designed 10 different prompt templates and selected the one with the highest average accuracy for use in the main text. Notably, previous studies have rarely explored AI-generated image detection using VLMs, making it impossible to directly adopt existing settings. Therefore, our approach represents a novel effort in optimizing prompt engineering for this task.

\section{Additional Results for RRBench}
In this section, we present the impact of different training datasets on detector performance and compare the results of the Human-Inspired In-Context Learning Approach with other in-context learning methods.

\subsection{Impact of Different Training Sets}
\label{train}

To further evaluate the best-performing detector on RRDataset, DRCT-ConvB \cite{chen2024drct}, and the most robust model, AIDE \cite{yan2024sanity}, we conduct additional testing on RRBench using the following model weights:

\noindent \textbf{For DRCT-ConvB\cite{chen2024drct}:}
\begin{enumerate}
    \item Trained on SDv1-4, with RRDataset fine-tuning
    \item Trained on SDv1-4, without RRDataset fine-tuning
    \item Trained on DRCT-2M, without RRDataset fine-tuning
    \begin{itemize}
        \item DRCT-2M is a large-scale dataset generated using advanced diffusion models, primarily SD XL. However, it differs from RRDataset, which uses SD 3.5 and FLUX as generators.
    \end{itemize}
    \item Trained on DRCT-2M, with RRDataset fine-tuning
\end{enumerate}

\noindent \textbf{For AIDE \cite{yan2024sanity}:}
\begin{enumerate}
    \item Trained on SDv1-4, with RRDataset fine-tuning
    \item Trained on SDv1-4, without RRDataset fine-tuning
\end{enumerate}

\noindent As shown in Tab. \ref{main_tab}, fine-tuning on RRDataset plays a crucial role in improving model performance. For DRCT-ConvB, fine-tuning on RRDataset led to a 33.67\% accuracy increase when pretrained on SDv1-4 and a 21.56\% increase when pretrained on DRCT-2M. Similarly, for AIDE, fine-tuning resulted in a 26.77\% improvement in accuracy.

The choice of pretraining datasets also significantly impacts performance. Without fine-tuning, the accuracy gap between DRCT-ConvB trained on DRCT-2M and SDv1-4 reached 12.71\%, indicating that larger and more advanced training datasets exhibit stronger transferability on RRBench. However, after fine-tuning, the accuracy difference between the two models shrank to just 0.69\%, suggesting that fine-tuning on a more advanced dataset can compensate for differences in pretraining data.

This finding implies that rather than continually expanding training datasets—which can be computationally expensive in terms of generation and retraining costs—similar performance gains may be achievable through targeted fine-tuning, making it a more efficient and scalable alternative for future AI-generated image detection improvements.

\begin{table*}[htbp]
\caption{Impact of Different Training Datasets on Model Accuracy.}
\label{main_tab}
\centering
\begin{tabular}{c|cc|cc|cc|c}
\toprule
\multirow{2}{*}{Model} & \multicolumn{2}{c|}{Original} & \multicolumn{2}{c|}{Transmission} & \multicolumn{2}{c|}{Re-digitization} & Overall \\
 & Fake(\%) & Real(\%) & Fake(\%) & Real(\%) & Fake(\%) & Real(\%) & ACC(\%) \\
\toprule
\rowcolor{gray!20}
\multicolumn{8}{c}{\textbf{DRCT-ConvB}} \\
SDv14- w finetune
 & 93.52 & 95.52
 & 92.82 & 95.09
 & 64.34 & 96.22
 & 89.59 \\
SDv14- w/o finetune
 & 53.64 & 58.21
 & 39.91 & 73.74
 & 51.42 & 54.99
 & 55.92 \\
 DRCT2M- w finetune
 & 95.15 & 94.09
 & 94.73 & 92.94
 & 68.35 & 96.42
 & \textbf{90.28} \\
 DRCT2M- w/o finetune
 & 68.00 & 73.42
 & 66.73 & 73.14
 & 49.74 & 80.74
 & 68.63 \\
 \rowcolor{gray!20}
 \multicolumn{8}{c}{\textbf{AIDE}} \\
SDv14- w finetune
 & 78.95 & 78.94
 & 74.72 & 78.75
 & 76.04 & 83.13
 & 78.42 \\
SDv14- w/o finetune
 & 56.04 & 61.69
 & 13.40 & 81.88
 & 28.78 & 68.10
 & 51.65 \\
\bottomrule
\end{tabular}
\end{table*}

\subsection{Comparisons with Other In-context Learning Strategies}
\noindent \textbf{Our Approch: } We observe a notable shift in human decision-making criteria when evaluating re-digitized and transmitted images. For re-digitization, over 25\% of participants attributed their judgments to lighting and reflection-related artifacts, while only 10\% considered image layout or realism as key factors. Conversely, for network transmission, factors such as sharpness, edges, and texture quality accounted for more than 52\% of responses.

In designing our in-context learning approach, we aim for VLMs to filter out potential confounding factors, such as compression artifacts from transmission and moiré patterns from screens and printed surfaces. To achieve this, we developed the following in-context learning template.

\begin{tcolorbox}[
    enhanced jigsaw,
    title=\textbf{Robustness-Oriented In-Context Learning},
    fonttitle=\bfseries,
    coltitle=black,
    colbacktitle=gray!15!white,
    colback=white,
    colframe=gray!70!black,
    arc=2mm,
    boxsep=2pt,
    left=2pt,
    right=2pt,
    top=2pt,
    bottom=2pt
]
\footnotesize
Act as a forensic image analyst specializing in origin classification. Analyze images through their intrinsic visual patterns while disregarding transmission/re-digitization artifacts. Focus on fundamental generation traces rather than secondary distortions.

\textbf{Contextual Examples:}
\begin{itemize}
    \item \textbf{[Transmitted Image]} Compressed JPEG with blocking artifacts, but shows consistent micro-textures in hair strands and natural skin pore variation → \textbf{Real}
    \item \textbf{[Transmitted Image]} Lossy blurred image with chromatic aberration, yet reveals perfect fractal patterns in the background and asymmetric eyelash duplication → \textbf{AI-generated}
    \item \textbf{[Re-digitized Image]} A scanned copy with a moiré pattern, but the content and details of the picture are real → \textbf{Real}
    \item \textbf{[Re-digitized Image]} Photographed print showing lens glare, yet contains Diffusion-typical floating specks and impossible light intersections → \textbf{AI-generated}
\end{itemize}

\textbf{Analysis Protocol:}
\begin{enumerate}
    \item \textbf{Primary Focus Areas:}
    \begin{itemize}
        \item Microscopic texture coherence (brush strokes/sensor noise patterns)
        \item Image content detail preservation beyond compression/scanning
        \item Biological imperfection consistency (asymmetric irises, skin translucency)
        \item Physical light interaction validity (shadow falloff, subsurface scattering, building material)
    \end{itemize}
    
    \item \textbf{Artifact Discounting:}
    \begin{itemize}
        \item Ignore format-specific compression patterns (JPEG blocking, slight color shift)
        \item Disregard scanning artifacts (dust particles, Newton rings)
        \item Overlook resampling distortions (aliasing, interpolation errors)
    \end{itemize}
    
    \item \textbf{Decisive Indicators:}
    \begin{itemize}
        \item AI-generated artifacts (e.g., diffusion-based oversmoothing, GAN-induced repetition, or hyperrealism)
        \item Anatomical plausibility under 3x digital magnification
        \item Material property consistency (metallic reflections, cloth draping)
    \end{itemize}
\end{enumerate}
\textbf{Output JSON:}
\begin{verbatim}
{ "classification": "AI-generated/Real" }
\end{verbatim}
\end{tcolorbox}

\noindent \textbf{CoT prompt for Comparison: }
\begin{tcolorbox}[
    enhanced jigsaw,
    title=\textbf{Chain-of-Thought (CoT) Prompt for AI-Generated Image Detection},
    fonttitle=\bfseries,
    coltitle=black,
    colbacktitle=gray!15!white,
    colback=white,
    colframe=gray!70!black,
    arc=2mm,
    boxsep=2pt,
    left=2pt,
    right=2pt,
    top=2pt,
    bottom=2pt
]
\footnotesize
\textbf{Task:} You are an expert in forensic image analysis. To determine whether an image is \textbf{AI-generated or real}, follow a structured reasoning process. Do not rely solely on immediate intuition; instead, break down your decision step by step.

\textbf{Step 1: Content Understanding \& Context}
\begin{itemize}
    \item What is the subject matter of the image? Describe its main elements (e.g., people, objects, background).
    \item Does anything seem out of place or conceptually inconsistent?
\end{itemize}

\textbf{Step 2: Fine-Grained Visual Inspection}
\begin{itemize}
    \item Examine details such as \textbf{textures, edges, and transitions}. Are there any \textbf{abnormal smoothness, inconsistencies, or unnatural repetitions}?
    \item Evaluate lighting and reflections—do they follow physical laws?
    \item Consider depth perception and perspective—is everything logically structured?
\end{itemize}

\textbf{Step 3: Logical Contradictions \& Anomalies}
\begin{itemize}
    \item Are there elements that should logically interact but do not (e.g., missing object shadows, disconnected reflections)?
    \item If the image contains humans, do facial features, hands, or expressions look \textbf{artificial or anatomically incorrect}?
    \item Does the image resemble known AI-generated artifacts (e.g., \textbf{diffusion-based oversmoothing, GAN-induced repetition, or hyperrealism})?
\end{itemize}

\textbf{Step 4: Final Reasoning \& Justification}
\begin{itemize}
    \item Summarize the strongest indicators supporting either classification.
    \item Make a final classification decision based on reasoning.
\end{itemize}

\textbf{Output Format (JSON):}
\begin{verbatim}
{ "classification": "AI-generated/Real", 
  "reasoning": "Step-by-step breakdown 
    of key factors influencing the decision"}
\end{verbatim}
\end{tcolorbox}

\noindent \textbf{Initial prompt for Comparison:} 

\begin{tcolorbox}[
    enhanced jigsaw,
    title=\textbf{Prompt for Vision-Language Models},
    fonttitle=\bfseries,
    coltitle=black,
    colbacktitle=gray!15!white,
    colback=white,
    colframe=gray!70!black,
    arc=2mm,
    boxsep=2pt,    % Reduce spacing inside the box
    left=2pt,      % Reduce left padding
    right=2pt,     % Reduce right padding
    top=2pt,       % Reduce top padding
    bottom=2pt     % Reduce bottom padding
]
\footnotesize
Act as an expert in computational photography and generative AI.
Analyze the visual characteristics to classify 
its origin as either real-world captured or AI-generated.

Your analysis should:

- Examine technical artifacts (unnatural textures, perfect symmetry, atypical shadow patterns)

- Check for common GAN/diffusion model fingerprints

- Evaluate biological plausibility (eyes, hair, skin textures)

- Identify hyperrealistic elements vs. physical-world imperfections

Format response as JSON: \{``classification": ``AI-generated/Real" \}
\end{tcolorbox}

\noindent \textbf{Comparison Results:} Tab. \ref{comparison} presents a comparison of four different prompting strategies. Our human-inspired Robustness-Oriented In-Context Learning achieves the best performance on 3 out of 4 VLMs, demonstrating its effectiveness in enhancing detection robustness, especially in challenging real-world conditions such as internet transmission and re-digitization.

The CoT+In-Context Learning approach achieves notable improvements on original images, suggesting that explicit reasoning chains help VLMs analyze fine details and generative traces more accurately when image quality is intact. However, its performance deteriorates significantly on transmitted and re-digitized images, indicating a strong reliance on pristine image quality. This suggests that CoT-based reasoning alone is insufficient to mitigate the impact of information loss, compression artifacts, and noise distortions introduced in real-world scenarios.

In contrast, our approch not only ensures higher robustness but also achieves the best overall performance across different VLMs, demonstrating that a robustness-oriented learning strategy is more effective in guiding VLMs to maintain high detection accuracy, even under degraded conditions.

\begin{table}[h]
\centering
\caption{Performance Comparison for Human-Inspired Robustness-Oriented In-Context Learning. }
\label{comparison}
\scalebox{0.8}{
\begin{tabular}{lcccc}
\toprule
 & \textbf{Original} & \textbf{Transmission} & \textbf{Redigital} & \textbf{ACC} \\
\rowcolor{gray!20}
\multicolumn{5}{c}{\textbf{Initial prompt}} \\
GPT-4o-latest & 92.94 & 84.71 & 73.08 & 83.58 \\
Claude-3.7-sonnet & 89.85 & 83.72 & 73.87 & 82.48 \\
Gemini-2-flash & 85.27 & 74.80 & 71.76 & 77.28 \\
Grok-2-vision & 68.99 & \textbf{73.08} & 64.82 & 68.96 \\
\rowcolor{gray!20}
\multicolumn{5}{c}{\textbf{Initial prompt + In-Context Learning (2-shot)}} \\
GPT-4o-latest & 91.85 & 84.06 & 74.55 & 83.49 \\
Claude-3.7-sonnet & 87.10 & 83.95 & 75.22 & 82.09 \\
Gemini-2-flash & 85.84 & \textbf{75.12} & 75.27 & 78.74 \\
Grok-2-vision & 67.28 & 72.86 & 66.71 & 68.95 \\
\rowcolor{gray!20}
\multicolumn{5}{c}{\textbf{CoT prompt + In-Context Learning (2-shot)}} \\
GPT-4o-latest & \textbf{96.27} & 83.58 & 71.45 & 83.77 \\
Claude-3.7-sonnet & 91.28 & 84.29 & 73.92 & 83.16 \\
Gemini-2-flash & \textbf{88.79} & 73.52 & \textbf{78.31} & \textbf{80.21} \\
Grok-2-vision & 71.02 & 71.47 & 65.93 & 69.47 \\
\rowcolor{gray!20}
\multicolumn{5}{c}{\textbf{Robustness-Oriented In-Context Learning (2-shot)}} \\
GPT-4o-latest & 95.67 & \textbf{88.17} & \textbf{78.58} & \textbf{87.47} \\
Claude-3.7-sonnet & \textbf{92.26} & \textbf{84.97} & \textbf{77.76} & \textbf{85.00} \\
Gemini-2-flash & 88.38 & 74.99 & 75.78 & 79.72 \\
Grok-2-vision & \textbf{72.86} & 71.52 & \textbf{71.43} & \textbf{71.94} \\
\bottomrule
\end{tabular}}
\end{table}

\section{Comparison of Human Attention Regions}
\subsection{Human Attention Map Generation}
\noindent \textbf{Data Collection: }
In this experiment, we select a set of images $\{I_1, I_2, \ldots, I_K\}$ for analysis. Each participant views the images on an screen and marks the Regions of Interest (ROIs) by drawing closed contours with a stylus. To ensure consistency, the following conditions should be met: The displayed images should have the same resolution and scaling across all participants.

\noindent \textbf{ROI Data Recording: }
Suppose there are $P$ participants. For each image $I_k$, participant $p$ (where $p=1,\ldots,P$) draws one or more closed polygons that represent their ROIs. We denote these polygons by
\[
\{\Omega_{p,k,1}, \Omega_{p,k,2}, \ldots\}.
\]
Each polygon $\Omega_{p,k,j}$ can be represented by a set of vertex coordinates, for example:
\[
\Omega_{p,k,j}
= \Bigl\{(x_{p,k,j,1},y_{p,k,j,1}), \ldots, (x_{p,k,j,n_j},y_{p,k,j,n_j})\Bigr\}.
\]

\noindent \textbf{Constructing the Binary Interest Mask: }
Each image $I_k$ has a size of $W \times H$. We define a matrix $M_{p,k}$ to represent participant $p$'s interest area on image $I_k$. Let the final set of aligned ROIs for participant $p$ on $I_k$ be $\{\Omega_{p,k,1}^*, \Omega_{p,k,2}^*, \ldots\}$. For any pixel $(x,y)$, we have:
\[
M_{p,k}(x,y)
=
\begin{cases}
1, & \text{if } (x,y) \in \Omega_{p,k,1}^* \cup \Omega_{p,k,2}^* \cup \ldots, \\
0, & \text{otherwise}.
\end{cases}
\]
$M_{p,k}(x,y) \in \{0,1\}$ defines a binary mask: $1$ indicates that pixel $(x,y)$ lies within the participant's drawn ROI, while $0$ indicates no interest in that pixel.

Then, we can compute an averaged mask:
\[
H_k(x,y)
= \frac{1}{P}
\sum_{p=1}^{P}
M_{p,k}(x,y).
\]
In this case, $H_k(x,y)$ lies within the interval $[0,1]$ and can be interpreted as the proportion that pixel $(x,y)$ is considered an ROI across all participants.

\noindent \textbf{Generating the Heatmap: }
To visualize  the averaged mask $H_k(x,y)$ we apply a color mapping that maps numerical values to colors and then overlay this heatmap on the original image. Typical steps include:
\begin{itemize}
    \item Rescale $H_k(x,y)$ from $[0,1]$ into the required color space.
    \item Adjust the transparency level to overlay the heatmap on the original image.
\end{itemize}
The resulting heatmap intuitively reveals which regions of the image draw higher or lower attention among the participant group.

\subsection{Result}
As shown in Fig. \ref{fig:attention} , participants in the original image group primarily focused on the main subject of the image, concentrating around the central area with minimal attention given to the edges and background. In the transmission group, participants also focused on the main subject, indicating that transmission did not significantly alter attention regions; the drop in accuracy here may be attributed to an overall reduction in image quality. However, in the re-digitization group, participants’ attention was more dispersed across the background, with less focus on the main subject. This shift suggests that re-digitization may lead to a diffusion of attention, likely contributing to the observed decrease in accuracy.

\begin{figure*}[htbp]
  \centering
  \includegraphics[width=0.9\textwidth]{attention_final.png}
  \caption{Comparison of Human Attention Regions in Original, Transmitted, and Re-digitized Images.}
  \label{conf}
  \label{fig:attention}
\end{figure*}

\section{Frequency Domain Analysis of Transmission and Re-digitization}
\label{f1}
To analyze the frequency characteristics of the images, we applied the Fast Fourier Transform (FFT) to convert the spatial-domain image $f(x, y)$ into its frequency-domain representation $F(u, v)$. The Fourier Transform decomposes the image into its sinusoidal components, with $|F(u, v)|$ representing the amplitude and $\angle F(u, v)$ the phase. The mathematical formulation of the 2D Fourier Transform is expressed as:

\begin{equation}
F(u, v) = \sum_{x=0}^{M-1} \sum_{y=0}^{N-1} f(x, y) \cdot e^{-j 2\pi \left(\frac{ux}{M} + \frac{vy}{N}\right)},
\end{equation}

where $(x, y)$ are pixel coordinates in the spatial domain, and $(u, v)$ are the corresponding frequency coordinates. For better visualization, we applied the FFT shift operation, which repositions the zero-frequency component (DC component) to the center of the spectrum. This is mathematically expressed as:

\begin{equation}
F_{\text{shifted}}(u, v) = F\left(u + \frac{M}{2}, v + \frac{N}{2}\right).
\end{equation}

The magnitude of the spectrum was computed as:

\begin{equation}
|F(u, v)| = \sqrt{\text{Re}(F(u, v))^2 + \text{Im}(F(u, v))^2}.
\end{equation}

To improve visualization, the magnitude spectrum was log-transformed to compress the dynamic range of the values. 
Finally, the spectrum was normalized to the range $[0, 1]$ for better contrast. Fig. \ref{fig:fre_real} and Fig. \ref{fig:fre_ai} illustrates the frequency-domain representation of the analyzed images.
% including the unshifted spectrum, shifted spectrum, and the log-scaled magnitude spectrum. 
It is evident that both transmission and re-digitization significantly alter the frequency domain characteristics of images, whether real or AI-generated. This alteration may explain the failure of frequency-dependent methods like Freq-Net and Fredect in detecting transmitted and re-digitized images.

\begin{figure*}[htbp]
  \centering
  \includegraphics[width=0.9\textwidth]{frq_real.png}
  \caption{Real Image Frequency Spectrum.}
  \label{fig:fre_real}
\end{figure*}

\begin{figure*}[htbp]
  \centering
  \includegraphics[width=0.9\textwidth]{freq_ai.png}
  \caption{AI Generated Image Frequency Spectrum.}
  \label{fig:fre_ai}
\end{figure*}

\section{Visualization of RRDataset.}
In this section, we present direct examples from RRDataset to illustrate its key characteristics. Fig. \ref{fig:exp1} and Fig. \ref{fig:exp2} showcase AI-generated special-scenario images, while Fig. \ref{fig:exp3} illustrates a comparison of images in their original, transmitted, and re-digitized states.

\begin{figure*}[htbp]
  \centering
  \includegraphics[width=0.90\textwidth]{example-1.png}
  \caption{Visualization of AI- Generated Special-Scenario Images.}
  \label{conf}
  \label{fig:exp1}
\end{figure*}

\begin{figure*}[htbp]
  \centering
  \includegraphics[width=0.90\textwidth]{example-2.png}
  \caption{Visualization of AI- Generated Special-Scenario Images.}
  \label{conf}
  \label{fig:exp2}
\end{figure*}

\begin{figure*}[htbp]
  \centering
  \includegraphics[width=0.95\textwidth]{example-3.png}
  \caption{Comparison of Original, Transmitted, and Re-digitized Images.}
  \label{conf}
  \label{fig:exp3}
\end{figure*}

\section{Further Discussion and Suggestion}
The rapid advancements in generative AI technologies have led to profound societal implications, especially in the context of AI-generated image detection. On one hand, these technologies offer creative opportunities, enhancing industries such as media, design, and entertainment. On the other hand, they pose significant challenges, including the spread of misinformation, digital forgeries, and potential misuse in sensitive domains like journalism, legal evidence, and intellectual property.

Our RRDataset provides a critical benchmark for evaluating the robustness of detection algorithms in real-world scenarios, directly addressing these challenges. By incorporating transmission and re-digitization into the dataset, we simulate practical conditions where AI-generated images are often manipulated. This ensures that detection methods are not only technically effective but also reliable in real-world scenarios.

Finally, by revealing robustness gaps in current detection methods, our work calls for the development of more generalized and resilient algorithms. This is essential not only for technical progress but also for fostering trust and accountability in AI-driven societies.

Based on the findings of our study, we propose the following recommendations:

\begin{enumerate}
    \item \textbf{For Researchers}: When developing new AI-generated image detectors, it is crucial to go beyond focusing solely on accuracy and consider their robustness in real-world scenarios. The integration of diverse features and leveraging human-like few-shot learning capabilities could be a promising direction for future advancements.
    
    \item \textbf{For Addressing the Trust Crisis}: Given the severe trust crisis currently emerging, especially in highly sensitive special-scenario images, skepticism towards authentic news content may significantly undermine the credibility and effectiveness of information dissemination.
    
    \item \textbf{For Generative Model Developers}: Considering the rapid pace of advancements in generative models, we recommend incorporating imperceptible watermarks into AI-generated content. This measure would ensure transparency and uphold people's right to know the origins of the content they encounter.
\end{enumerate}

\section{Limitation}
\textbf{Benchmark Limitations:} Although we have endeavored to include as many detection methods as possible, including the latest works from KDD 2025, AAAI 2025, and ICLR 2025, some proprietary methods could not be incorporated into RRBench. Additionally, it is possible that newer open-source detectors have not yet been included. We are committed to continuously updating and curating detection methods in future iterations.

\noindent \textbf{Dataset Limitations:} RRDataset includes some of the latest and most powerful generative models. However, newer and more advanced models will likely continue to emerge, which may not be represented in RRdataset. To address this, we plan to update the RRDataset continuously in the future.
